# Supplementary material for: Multimodal Reasoning Agent for Zero-Shot Composed Image Retrieval
Source: arXiv:2505.19952 source file (2025-05-26)
Supplement: Supplementary file 1 [file experiment_setup.tex]

\section{Experimental Setup\label{app:experimental_setup}}
\paragraph{Evaluated Models}
We evaluate the capabilities of some advanced open-source and closed-source LLMs and MLLMs for M$^2$RAG task. The involved models are listed in Table \ref{tab:baseline_models}.
Besides, we also implement a separate approach, \textit{i.e.,} the MuRAR method with GPT-4o as the backbone model~\cite{zhu2024murar}.

\begin{table}[h]
    \centering
    \resizebox{1.0\linewidth}{!}{
        \begin{tabular}{cc}
        \toprule
            \textbf{LLM} & \textbf{MLLM} \\
        \midrule
            GPT-4o & GPT-4o \\
            Llama-3.1-70B-Instruct & Llama-3.2-90B-Vision-Instruct \\
            Llama-3.1-8B-Instruct & Llama-3.2-11B-Vision-Instruct \\
            Qwen-2.5-72B-Instruct & Qwen-2-VL-72B-Instruct \\
            Qwen-2.5-7B-Instruct & Qwen-2-VL-7B-Instruct \\
        \bottomrule
        \end{tabular}
    }
    \caption{\label{tab:baseline_models}LLMs and MLLMs used for M$^2$RAG task.}
\end{table}

\paragraph{Implementation Details}
For the generation process, we deployed open-source LLMs and MLLMs using vLLM~\cite{kwon2023efficient} on Nvidia A100-SXM4-80GB GPUs. Models with 7B-11B parameters operate on a single GPU, while those exceeding 70B parameters are distributed across 4 GPUs using tensor parallelism. The context length is configured at 64k for the Llama series and 32k for the Qwen series.
During generation, we use a top-$k$ selection method with $k$ set to 20 for filtering text elements from each webpage. The maximum number of auxiliary and web page specific images is restricted to 5, with a total input image cap at 10. Images are resized to 512 $\times$ 512 thumbnails for MLLMs processing.
For evaluation, we implemented our customized metrics using the GPT-4o model to ensure the robust comprehensive assessment. 
Besides, the RAG metrics are implemented with RAGAS~\cite{es2023ragasautomatedevaluationretrieval} by using the GPT-4o-mini model.
